# Supplementary material for: Ontology-Guided Query Expansion for Biomedical Document Retrieval using Large Language Models
Source: arXiv:2508.11784 source file (2025-08-15)
Supplement: Supplementary file 1 [file g_appendix.tex]

\appendix
\section{Prompt Templates for Ontology-Guided Query Expansion}

\subsection{Biomedical Entity Recognition}

\begin{center}
\begin{tcolorbox}[
  colback=blue!5,
  colframe=blue!20,
  title=Medically Relevant Term Extraction,
  fonttitle=\bfseries,
  coltitle=black,
  boxrule=0.8pt,
  arc=4pt
]

\textbf{System Prompt}
\begin{tcolorbox}[mypromptbox]
You are a biomedical information retrieval assistant.
\end{tcolorbox}

%\vspace{0.4em}

\textbf{User Prompt}
\begin{tcolorbox}[mypromptbox]
Your task: Extract key medical terms from the query. If the query lacks significant medical terms, return an empty list.

\end{tcolorbox}

%\vspace{0.4em}

\textbf{In-Context Examples}
\begin{tcolorbox}[mypromptbox]
Query: Dietary Treatment of Crohn's Disease \\
Terms: [Dietary Treatment, Crohn's Disease]

Query: Neurobiology of Artificial Sweeteners \\
Terms: [Neurobiology, Artificial Sweeteners]

Query: Boosting Good Bacteria in the Colon Without Probiotics \\
Terms: [Good Bacteria, Probiotics]

Query: Veggies vs. Cancer \\
Terms: [Cancer]

Query: Native Americans \\
Terms: []
\end{tcolorbox}

%\vspace{0.4em}

\textbf{Input Query}
\begin{tcolorbox}[mypromptbox]
Query: \{query\} \\
Terms: [...]
\end{tcolorbox}

\end{tcolorbox}
\end{center}

For the biomedical term extraction task, we prompt the LLM using five in-context examples that demonstrate the desired input-output behavior. To ensure consistent formatting of the model's output---particularly for \texttt{LLaMA 3}---we append an explicit constraint to the instruction,

\begin{quote}
\ttfamily
Strictly follow the output format. \\
Output format: \\
Terms: [term1, term2, ...]
\end{quote}
